# Supplementary material for: Divining the Shape of Nascent Polymer Crystal Nuclei
Source: arXiv:1908.01735 ancillary file (2019-08-05)
Supplement: Supplementary file 1 [file SupportingInformation.pdf]

# Divining the Shape of Nascent Polymer Crystal Nuclei

## Supporting Information

Kyle Wm. Hall,[1,2,3,a)] Timothy W. Sirk,[4] Simona Percec,[1] Michael L. Klein,[1,2] and Wataru Shinoda[3]

[1)] *Department of Chemistry, Temple University, Philadelphia, Pennsylvania 19122, United States*

[2)] *Institute for Computational Molecular Science, Temple University, Philadelphia, Pennsylvania 19122, United States*

[3)] *Department of Materials Chemistry, Nagoya University, Furo-cho, Chikusa-ku, Nagoya 464-8603, Japan*

[4)] *U.S. Army Research Laboratory, Aberdeen Proving Ground, Maryland 21005, United States*

[a)] Electronic mail: k.wm.hall@temple.edu

*The reference list at the end of the main body text provides the bibliographic information for ref. 1-63. Ref. 64-69 appear at the end of this document.*

## METHODOLOGICAL DETAILS

### A. System Preparation and Simulation Details

The starting configurations for the crystallization simulations at 285 K were obtained using the identical protocol as for the 270 K crystallization simulations in our previous study.[6] A high-level conceptual description is provided here; see ref. 6 for complete details. Briefly, a melt composed of 400 $n$-$C_{720}H_{1442}$ chains was prepared and equilibrated at 500 K and 1 atm. Ten configurations were selected from a subsequent production simulation of the melt. The selected configurations were used to launch ten separate simulations at 300 K, thus yielding ten metastable $n$-$C_{720}H_{1442}$ melts below the melting temperature of SDK polyethylene chains, which is expected to be $\sim$400 K.[46] The final configurations from the 300 K simulations were used to launch the ten 285 K simulations of this study.

The methodological details for the 285 K crystallization simulations were very similar to the 270 K crystallization simulations in our previous study.[6] This study's isobaric-isothermal (NPT) crystallization simulations were conducted using LAMMPS.[64] The simulations had periodic boundary conditions. A 15.0 Åcutoff was used when calculating Lennard-Jones interactions. Particle positions were evolved according the approach of Shinoda and coworkers[65] while pressure was maintained at 1 atm with anisotropic chain barostat (4-member chains, 10-ps coupling constants), and temperature was maintained at 285 K with Nosé-Hoover[66,67] chain thermostats[68] (4-member chains, 1-ps coupling constants). The simulations used a 5 fs time step, and each simulations was 200,000,000 time steps in length. Previous work has demonstrated that SDK polyethylene chains

diffuse approximately fourfold faster than their experimental counterparts.[6,46] As such and similar to previous work,[6,46] all simulation times were scaled post hoc by a factor of 4.07. The 5-fs time step used in the LAMMPS simulations thus corresponded to 20.35 fs. All times reported in the main body text are scaled times that include the factor of 4.07. During each simulation, system properties and configurations were saved every 5,000 and 20,000 time steps, respectively.

## B. Assessing Alignment & Crystallinity

For the crystallization simulations, the crystallinity of individual coarse-grain beads was determined according to the local alignment between polymer chains as revealed by the $P_2$ order parameter, which has been extensively used in the polymer literature to distinguish crystalline and non-crystalline polymer chain segments and phases in polyethylene systems (*e.g.,* see ref. 5,6,13,43,59). Consistent with previous work leveraging the SDK model to study polyethylene,[6,46] the following procedure was used when estimating $P_2$ values and assigning crystallinity.

1. For each non-terminal bead, the direction of its polymer chain backbone was estimated using a unit vector ($u$) with the same direction as the vector between the two intramolecular neighbors of the bead. For terminal beads, the direction of $u$ was estimated using the bond vector of the bead.

2. For each bead ($i$), the angles ($\Theta$) between its backbone vector ($u$) and those of its neighbors were determined for all neighbours within 6.35 Å of bead $i$. The distance cutoff is the second minimum in the radial distribution function for SDK polyethylene crystals.[6]

3. Using the extracted angles, the $P_2$ order parameter for bead $i$ was calculated according to:

$$P_2(i) = \langle (3cos^2\Theta - 1)/2 \rangle \tag{1}$$

where the angular brackets indicate averaging over all of the neighbors within 6.35 Å of bead $i$.

4. Beads with $P_2 \geq 0.85$ were labelled crystalline.[6,46]

Crystalline clusters were extracted from each simulation configuration by performing cluster analysis on its crystalline beads. Beads within 6.35 Å were considered to be part of the same cluster.

## C. Estimate of Critical Nucleus Size

Previous work indicates that the critical nucleus size coincides with a minimum in the distribution $v * p(v)$ where $v$ is nucleus volume and $p(v)$ is the corresponding population.[5] Given that a particle-based definition of nucleus size was leveraged in this study, $v * p(v)$ was approximated using the function $V(n) * P(n)$ where $V(n)$ is the average volume of a cluster of size $n$ and $P(n)$ is the probability of a cluster of size $n$. Voronoi tessellations were used to estimate cluster volumes. For the 285 K crystallization simulations used in this study, $V(n) * P(n)$ yielded a critical nucleus estimate of ∼600 carbon atoms (see Fig S1).

Given that the connection between $v * p(v)$ and critical nucleus size has been demonstrated only under the assumptions of classical nucleation theory,[5] an alternative strategy was also leveraged to estimate the critical nucleus size for the polyethylene model and crystallization conditions used in this study. More specifically, a probability distribution was constructed for cluster size using only the crystalline clusters extracted from the non-nucleating simulations, specifically those simulations that did not exhibit the

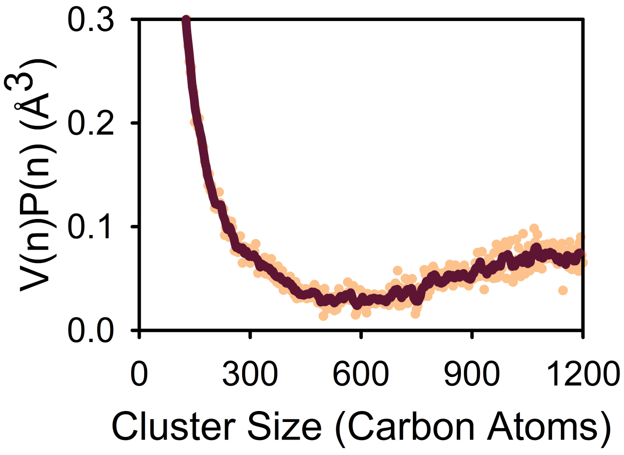


FIG. S1. The joint size-probability function $V(n) * P(n)$ for crystalline clusters extracted from the simulations. The red line corresponds to a rolling average with a period of 9 carbon atoms to guide the eyes. The orange points are the underlying raw data.

potential energy decrease characteristic of polyethylene crystallization during their ∼4-$\mu$s window (see the inset to Fig. 1C). The probability distribution decays rapidly and reaches zero well before 600 carbon atoms. In particular, for the non-nucleating simulations, the largest cluster ever observed corresponded to 456 carbon atoms, placing an approximate lower bound on the critical nucleus size. The conclusions of this study depend only on the approximate size of critical nuclei (*i.e.,* between ∼450 and ∼600 carbon atoms), and are robust with respect to the exact critical nucleus size.

## D. Radius of Gyration Tensor & Shape Metrics

Cluster shapes were quantified based on the metrics introduced by Theodorou and Suter for studying polymers.[48] See ref. 48 for additional details and further discussion. The radius of gyration tensor for a cluster of particles is given by

$$S = \langle rr \rangle \tag{2}$$

where $r$ is the position of a particle with respect to the geometric center of the cluster, $rr$ is its dyadic product, and the angular brackets indicate an average over all of the particles composing the cluster. The eigenvectors of $S$ correspond to a principal axis system for the cluster. As detailed in the main body text, the axes and eigenvalues ($\lambda$) were labeled according to the convention $\lambda_{major} \geq \lambda_{median} \geq \lambda_{minor}$. Given that the eigenvalues sum to $R_g^2$, the $b_{rel}$ and $c_{rel}$ values of each cluster were calculated according to:

$$b_{rel} = [\lambda_{major} - 0.5(\lambda_{median} + \lambda_{minor})]/R_g^2 \tag{3}$$

$$c_{rel} = (\lambda_{median} - \lambda_{minor})/R_g^2 \tag{4}$$

Equation 3 and 4 correspond to the $b$ and $c$ metrics introduced by Theodorou and Suter[48] normalized by $R_g^2$ in order to enable shape comparisons across clusters of differing size. The $\kappa^2$ of each cluster was also determined, and is related to $b_{rel}$ and $c_{rel}$ according to:

$$\kappa^2 = b_{rel}^2 + 0.75 c_{rel}^2 \tag{5}$$

Details about interpreting $b_{rel}$, $c_{rel}$, and $\kappa^2$ values are provided in the caption to Fig. 2.

## E. Fractal Dimension

The fractals dimension of clusters were extracted based on previously described box-counting approaches[59,69] with some minor revisions based on the specifics of the systems considered in this study (*e.g.,* cutoffs based on the size of the coarse-grain beads used in this study).

1. For each cluster, the positions of its constituent particles were converted to a local frame of reference. The local frame of reference was a 3D Cartesian system with axes corresponding to the three eigenvectors of the cluster's radius of gyration tensor, and with an origin corresponding to the the center of mass of the cluster.

2. The absolute distance of each particle along each axis was determined.

3. The maximum of distance extracted in Step 2 ($L_{max}$) was used to construct a bounding box around the nucleus ranging from $-L_{max}$ to $L_{max}$ along each axis, and with a side length of $L_{box} = 2L_{max}$.

4. The bounding box of side length was sequentially subdivided into finer meshes composed of cubic voxels with side lengths $L_{side} = L_{box}, L_{box}/2, L_{box}/4, ...$ until $L_{side}$ was less than $\sim$1.13 Å (*i.e.,* $R_{bead}/4$ where $R_{bead}$ is the radius of the coarse-grain beads used to represent polyethylene in this study). For each voxel mesh (*i.e.,* each $L_{side}$), the number of voxels intersecting with the constituent particles of the cluster ($N_{intersect}$) was determined. A voxel was deemed to be intersecting a particle if the center of the voxel and the particle were separated by less than $L_{side}/2 + R_{bead}$ along each axis of the local frame.

5. The fractal dimension of the cluster was taken to be the slope of the linear fit of $-ln(N_{intersect})$ as a function of $ln(L_{side})$ ($R^2$>0.99).

The above procedure was performed on all clusters corresponding to 600 carbon atoms.

## F. Nematic Director

The overall direction of the stems composing each clusters was assessed by estimating the nematic director of the cluster according to the procedure of Eppenga and Frenkel[63] as is briefly summarized here. For each cluster, the order tensor $Q$ was calculated according to:

$$Q = \left\langle \frac{3}{2} uu - \frac{1}{2} I \right\rangle \tag{6}$$

where $uu$ is the dyadic product of the backbone orientation vector $u$ of a constituent bead with itself, $I$ is a 3 by 3 identity tensor, and the angular brackets indicate an average over all of the beads composing the cluster. The nematic director of the cluster was then the eigenvector associated with the largest eigenvalue of $Q$.

## REFERENCES


[64] S. Plimpton, Journal of Computational Physics **117**, 1 (1995).

[65] W. Shinoda, M. Shiga, and M. Mikami, Phys. Rev. B **69**, 134103 (2004).

[66] S. Nosé, Molecular Physics **52**, 255 (1984).

[67] W. G. Hoover, Phys. Rev. A **31**, 1695 (1985).

[68] G. J. Martyna, M. L. Klein, and M. Tuckerman, J. Chem. Phys. **97**, 2635 (1992).

[69] J. Gagnepain and C. Roques-Carmes, Wear **109**, 119 (1986).
